# Supplementary material for: Distribution Alignment: A Unified Framework for Long-tail Visual Recognition
Source: arXiv:2103.16370 source file (2021-03-30)
Supplement: Supplementary file 1 [file supp.tex]

\section{Supplementary}

\subsection{Image Classification on ImageNet-LT}

\begin{table*}[h!]

\centering
\caption{\textbf{Quantitative results on ImageNet-LT:} All models use the feature extractor trained with 90 epoch(except the models marked with \textbf{F-200e}, which means the feature extractors are trained with 200 epoch, $\dagger$ means the model uses cosine classifier. All our methods are reported with 95\% confidence interval over 10 runs.}
\vspace{-0.8em}
% \begin{threeparttable}
 \resizebox{0.99\textwidth}{!}{
\begin{tabular}{l|c|l|lll|l|lll}
\toprule
\multirow{2}{*}{\textbf{Method}}  & \multirow{2}{*}{\textbf{Align}} & \multicolumn{4}{c|}{\textbf{Top-1 Accuracy@R-50}} & \multicolumn{4}{c}{\textbf{Top-1 Accuracy@X-50}}  \\
\cmidrule{3-10}
                                  &             &\textbf{Average} & \textbf{Many } & \textbf{Medium } & \textbf{Few } &\textbf{Average} & \textbf{Many } & \textbf{Medium } & \textbf{Few } \\
\midrule
Naive\cite{kang2019decoupling}    & -           & 41.6	           & 64.0           &    33.8         &  5.8           & 44.4	          & 65.9           &       37.5     &  7.7 \\
%Cosine                            & -           & 48.4             &  68.4          &    41.8         &  15.2          & 49.2        &  68.9               &    42.8     & 15.6\\
\midrule
cRT\cite{kang2019decoupling}          & Learnable   & 47.3             & 58.8           &    44.0         &  26.1         &  49.6        & 61.8          &        46.2    &   27.4\\
cRT$^\dagger$                         & Learnable   & -                & -              &    -            &   -           &  49.7        & 60.4          &        46.8    &   29.3\\
LWS\cite{kang2019decoupling}          & Learnable   & 47.7             & 57.1           &    45.2         &  29.3         &  49.9        & 60.2          &        47.2    &   30.3  \\
NCM\cite{kang2019decoupling}          & Hand-Craft  & 44.3             & 53.1           &    42.3         &  26.5         & 47.3         & 56.6          &        45.3    &   28.1\\
$\tau$-Norm\cite{kang2019decoupling}  & Hand-Craft  & 46.7             & 56.6           &    44.2         &  27.4         & 49.4         & 59.1          &        46.9    &   30.7    \\
Logit Adjust\cite{}                   & Hand-Craft  & 50.3             & -              &      -          &   -           &            - & - &- &-\\
Deconfound$^\dagger$\cite{}           & Hand-Craft  &  -               & -              &      -          &   -           & 51.8            & 62.7       &        48.8    &   31.6\\
\midrule
%Naive$^\dagger$   & - & 45.2        &  67.4               &    38.0    & 7.5  \\
%Cosine$^\dagger$  & - & R-50 & 48.4        &  68.4               &    41.8    & 15.2   \\
%Naive-Bound                           &  -          & 56.1             & 62.3           &   53.6          & 47.6\\
\textbf{DisAlign}                     &  Learnable  &  51.29\colorpm{$\pm 0.03$}  &  59.90\colorpm{$\pm 0.04$} &  49.91\colorpm{$\pm 0.05$}  &  31.76\colorpm{$\pm 0.10$}      
                                                    &  52.49\colorpm{$\pm 0.03$}  &  61.54\colorpm{$\pm 0.03$} &  50.73\colorpm{$\pm 0.07$}  &  33.05\colorpm{$\pm 0.09$}\\
\textbf{DisAlign$^\dagger$}           &  Learnable  &  52.90\colorpm{$\pm 0.03$}  &  61.33\colorpm{$\pm 0.04$} &  52.24\colorpm{$\pm 0.05$}  &  31.36\colorpm{$\pm 0.07$}
												    &  53.40\colorpm{$\pm 0.02$}  &  62.73\colorpm{$\pm 0.07$} &  52.14\colorpm{$\pm 0.05$}  &  31.44\colorpm{$\pm 0.14$}\\
\midrule
\textbf{DisAlign}\small(F-200e)      &  Learnable   &  53.68\colorpm{$\pm 0.03$} &   63.13\colorpm{$\pm 0.05$} &  51.46\colorpm{$\pm 0.06$}  &  34.74\colorpm{$\pm 0.08$}   \\
\textbf{DisAlign$^\dagger$}\small(F-200e)&  Learnable &53.61\colorpm{$\pm 0.03$} &   63.95\colorpm{$\pm 0.03$} &  51.74\colorpm{$\pm 0.04$}  &  30.89\colorpm{$\pm 0.09$} \\
%\textbf{DisAlign$^\dagger$}\small(F-200e)   &  Learnable  &  \textbf{52.7} & 65.2 & \textbf{49.7} & 27.6 \\
%\midrule
%Naive$^\dagger$     & - & 45.2        &  67.4               &    38.0    & 7.5  \\
%Naive+SA$^\dagger$     & - & 48.4        &  68.4               &    41.7    & 15.5  \\
%\textbf{DisCal-Naive}  & & R-50 &  Learnable     &  51.7 & 62.3 & 48.7 & \textbf{32.1}   \\
%\textbf{DisCal-Cosine} & & R-50 &  Learnable  &  \textbf{52.7} & 65.2 & \textbf{49.7} & 27.6 \\
%\midrule
%cRT$^\dagger$\cite{kang2019decoupling}   & Learnable& 52.8   &   65.8  & 49.1 & 28.9  \\
%Cosine\cite{} & X-50 & 47.6 & 67.3 & 41.3 & 14.0\\
%\midrule
%Naive$^\dagger$   & X-50     & 46.8        &  68.1               &    40.2    & 9.3   \\
%Cosine$^\dagger$  & X-50     & 49.2        &  68.9               &    42.8    & 15.6  \\
\bottomrule
\end{tabular}} %\end{threeparttable}
\label{tab:classification}
\end{table*}

\subsection{Semantic Segmentation}

\paragraph{Dataset.} ADE20K dataset is a scene parsing benchmark, which contains 150 stuff/object categories. The dataset includes 20K/2K/3K images for training, validation and testing. Compared with the image classification\cite{liu2019large}, the imbalance of ADE20K is more serve than the image classification, which has a imbalance ratio of \textbf{788}(Max/Min). Follow the similar protocol in image classification, we divide the 150 categories into 3 groups according to ratio of pixel number over whole dataset. Specifically, three disjoint subsets are: \textit{head classes}(classes each with a ratio over 1.0\%), \textit{body classes}(classes each with a ratio ranging from 0.1\% to 1\%) and \textit{tail classes}(classes under a ratio of 0.1\%), complete list of the split is reported in supplementary material.

\paragraph{Implementation Details.} We implement our method based on MMSegmentation toolkit\cite{}. In the representation learning training phase, we set the learning rate to 0.01 initially, which gradually decreases to 0 by following the 'poly' strategy as \cite{zhang2018context}. The images are cropped to $512\times 512$ and augmented with randomly scaling(from 0.5 to 2.0) and flipping. ResNet-50, ResNet-101 and ResNeSt-101 are used as the backbone. For the evaluation metric, we use the mean Intersection of Union(mIoU) and pixel accuracy(pixelAcc). All models are trained with 160k iterations with a batch size of 32 based on 8 V100 GPUs. In the DisAlign stage, we follow the similar protocol as the stage-1 and only training the model with 8k iterations.

\subsection{Object Detection}
\begin{table*}
\caption{\textbf{Results of Mask R-CNN FPN with different backbone:}We denote \textbf{RS} for resampling image. All experiments results are evaluated on the LVIS 0.5 validation set with the score threshold at 0.0001. ($*$ means we use Forest R-CNN without NMS resampling for fair comparsion).}
\label{tab:maskrcnn}
\vspace{-0.8em}
\centering
    \resizebox{0.98\textwidth}{!}{
\begin{tabular}{l|l|c||c||ccc||c||ccc}
\toprule
B & Method & Pre-Train & $\text{mAP}_{box}$ & $\text{mAP}_{box}^r$ & $\text{mAP}_{box}^c$ & $\text{mAP}_{box}^f$ & $\text{mAP}_{seg}$& $\text{mAP}_{seg}^r$ & $\text{mAP}_{seg}^c$ & $\text{mAP}_{seg}^f$ \\
\midrule
\multirow{14}{*}{\rotatebox{90}{Mask R-CNN + R-50}}   & Mask R-CNN 	&\multirow{8}{*}{ImageNet}	 & 20.8 &  3.3  &  19.5 & 29.4     & 21.2 & 3.7 & 21.6 & 28.4  \\
& Mask R-CNN$^\dagger$ 	     &             & 22.8 &  10.2 &  21.1 & 30.1     & 23.8 & 11.5 & 23.7 & 28.9 \\
& Forest R-CNN$^*$\cite{}		 &             & 24.0 & - & - & - & 23.6 & 10.9 & 24.4 & 27.5 \\
& SimCal\cite{}				 &             & 22.6 & 13.7 & 20.6 & 28.7  & 23.4 & 16.4 & 22.5 & 27.2 \\
& RFS\cite{}				 &             & 23.6 &	 12.8 & 22.3 & 29.4 & 24.3 & 14.6& 24.0 & 28.5\\
& EQL\cite{}				 &             & 23.6 &  8.5  & 23.9 & 29.3 & 24.0 &  9.4 & 25.2 & 28.4 \\
\cmidrule{2-2}\cmidrule{4-10}
& \textbf{DisAlign}           &            & 23.9 & 7.5  & 25.0 & 29.1  & 24.3 & 8.5 & 26.3 & 28.1\\
& \textbf{DisAlign$^\dagger$} &            & \textbf{25.6} &  13.7 & 25.6 & 30.5 & 26.3 & 14.9 & 27.6 &  29.2 \\
\cmidrule{2-10}
& Mask R-CNN 			  &  \multirow{6}{*}{COCO} 	& 22.8 &  2.6  &  21.8 & 32.0     & 23.9 & 2.8 & 23.4 & 30.5  \\
& Mask R-CNN$^\dagger$ 	  &                         & 25.0 &  10.2  & 23.9 & 32.3     & 25.3 & 11.0 & 25.5 & 30.7 \\
%\cmidrule{1-2}\cmidrule{4-10}
%& RFS\cite{gupta2019lvis}  &   &    & \\
%EQL\cite{gupta2019lvis}  & & 	& - & - &  - & - & 24.4 & 14.5& 24.3 & 28.4 \\
%Forest R-CNN	 		 & &   								& 25.9 & 16.9 & 26.1 & 29.2       & 25.6 & 18.3 & 26.4 & 27.6\\  
& GroupSoftmax             &      & 25.8 & 15.0 & 25.5 & 30.4       & 26.3 & 18.0 & 26.9 & 28.7 \\
%SimCal\cite{}            & &                                  & 22.6 & 13.7   & 20.6 & 28.7     & 23.4 & 16.4 & 22.5 & 27.2 \\
\cmidrule{2-2}\cmidrule{4-10}
& \textbf{DisAlign}           &    &    25.5 & 8.2 & 26.3 & 32.4 & 25.7 & 9.4 & 27.6 & 29.7 \\
& \textbf{DisAlign$^\dagger$} &    &	 27.6 & 14.8   & 27.9 & 32.4    & 27.9 & 16.2 & 29.3 & 30.8\\
\midrule
\midrule
% ResNet-101
\multirow{10}{*}{\rotatebox{90}{Mask R-CNN + R-101}}   & Mask R-CNN 	&\multirow{6}{*}{ImageNet}	 & 	22.3 &	2.6	& 21.1	& 31.6 &	22.6 &	2.7	& 22.8 &	 30.2\\
&Mask R-CNN$^\dagger$ 		     & 	   & 	24.5 & 	10.1 & 23.2 & 	31.8 & 	25.0 & 	11.2 & 25.2 & 	30.4\\
%\midrule
&RFS\cite{gupta2019lvis}      & 	& 26.1 & 15.2&	25.3 &	31.4 &	26.2 &	15.9 &	26.4 &	30.0\\
& EQL\cite{gupta2019lvis}     &     & 25.9 & 9.2 &  26.9 & 31.1 & 25.9 & 10.0 & 27.9 & 29.8 \\
\cmidrule{2-2}\cmidrule{4-10}
&\textbf{DisAlign}            &     & 25.5 & 9.0 & 26.5 & 30.9 &  25.8 & 10.3 & 27.6 & 29.6  \\
&\textbf{DisAlign$^\dagger$}  &     & 27.5 & 15.9 & 27.5 & 32.0 & 28.2 & 17.8 & 29.7 & 30.5\\
\cmidrule{2-10}
&Mask R-CNN 			& \multirow{5}{*}{COCO}    	& 	24.3 &	3.9 &		23.0 &		34.1 &		24.3 &		4.1 &		24.2 &		32.3 \\
&Mask R-CNN$^\dagger$   &     & 27.1	& 11.2 &	26.2&	34.4&	27.2	& 13.0	& 27.7 &	33.4  \\
%\cmidrule{1-2}\cmidrule{4-10}
%&RFS\cite{gupta2019lvis}  &  COCO  &    & \\
%EQL\cite{gupta2019lvis}  & & 	& - & - &  - & - & 24.4 & 14.5& 24.3 & 28.4 \\
%Forest R-CNN	 		 & &   								& 25.9 & 16.9 & 26.1 & 29.2       & 25.6 & 18.3 & 26.4 & 27.6\\  
%&GroupSoftmax             &       & 25.8 & 15.0 & 25.5 & 30.4       & 26.3 & 18.0 & 26.9 & 28.7 \\
%SimCal\cite{}            & &                                  & 22.6 & 13.7   & 20.6 & 28.7     & 23.4 & 16.4 & 22.5 & 27.2 \\
\cmidrule{2-2}\cmidrule{4-10}
&\textbf{DisAlign}           &    &  27.0 & 9.3 &  27.8 & 33.1 & 26.9 & 10.5 & 28.6 & 31.4    \\
&\textbf{DisAlign$^\dagger$} &    &  30.0 & 19.3 & 30.0 & 34.2 & 30.0 & 20.6 & 31.3 & 32.2      \\
\midrule
\midrule 
% ResNeXt-101
\multirow{10}{*}{\rotatebox{90}{Mask R-CNN + X-101}}   & Mask R-CNN 	&\multirow{6}{*}{ImageNet}	 & 24.4 & 3.9 & 24.1 & 33.1 & 25.0 & 4.2 & 26.3 & 31. \\
&Mask R-CNN$^{cos}$ 		     & 	   & 	26.9 &	12.1  &	26.1  &	33.8  &	27.7  &	15.2  &	28.2  &	32.2 \\
%\midrule
&RFS\cite{gupta2019lvis}         & 	   & 26.7 & 15.5 & 25.7 & 32.5 & 27.1 & 16.8 & 27.0 & 32.4    \\
& EQL\cite{gupta2019lvis}        &     &     \\
\cmidrule{2-2}\cmidrule{4-10}
&\textbf{DisAlign} &      &    \\
&\textbf{DisAlign$^\dagger$} &    \\
\cmidrule{2-10}
&Mask R-CNN 				& \multirow{5}{*}{COCO}  & 26.7 &  6.4 & 26.5 & 35.0 &	26.4 &	7.0	 &  27.2 &	33.1 \\
&Mask R-CNN$^\dagger$ 	    &                        & 28.9 & 12.1 & 28.9 &	35.6 &	28.9 &	13.4 & 	30.1 & 	33.6  \\
\cmidrule{2-2}\cmidrule{4-10}
&\textbf{DisAlign}           &          \\
&\textbf{DisAlign$^\dagger$} &            \\
%\midrule
%\midrule 
\bottomrule
\end{tabular}}
\end{table*}

\newpage
\subsubsection{Overall}

\begin{table*}
\caption{\textbf{Results of Mask R-CNN FPN with different backbone:}We denote \textbf{RS} for resampling image. All experiments results are evaluated on the LVIS 0.5 validation set with the score threshold at 0.0001. ($*$ means we use Forest R-CNN without NMS resampling for fair comparsion).}
\label{tab:maskrcnn}
\vspace{-0.8em}
\centering
    \resizebox{0.98\textwidth}{!}{
\begin{tabular}{l|c||c||ccc||c||ccc}
\toprule
Method & Backbone & $\text{mAP}_{box}$ & $\text{mAP}_{box}^r$ & $\text{mAP}_{box}^c$ & $\text{mAP}_{box}^f$ & $\text{mAP}_{seg}$& $\text{mAP}_{seg}^r$ & $\text{mAP}_{seg}^c$ & $\text{mAP}_{seg}^f$ \\
\midrule
Mask R-CNN 					&	\multirow{7}{*}{R-50} 		& 22.8 &  2.6  &  21.8 & 32.0     & 23.9 & 2.8 & 23.4 & 30.5  \\
Mask R-CNN$^\dagger$ 	    &		                        & 25.0 &  10.2  & 23.9 & 32.3     & 25.3 & 11.0 & 25.5 & 30.7 \\
%\midrule
RFS\cite{gupta2019lvis}  &    & \\
EQL\cite{gupta2019lvis}  & 	& - & - &  - & - & 24.4 & 14.5& 24.3 & 28.4 \\
Forest R-CNN$^*$	 		 &   								& 24.0 & - & - & - & 23.6 & 10.9 & 24.4 & 27.5\\  
GroupSoftmax             &                                  & 25.8 & 15.0 & 25.5 & 30.4       & 26.3 & 18.0 & 26.9 & 28.7 \\
SimCal\cite{}            &                                  & 22.6 & 13.7   & 20.6 & 28.7     & 23.4 & 16.4 & 22.5 & 27.2 \\
\midrule
\textbf{DisAlign}           &  \multirow{2}{*}{R-50}         \\
\textbf{DisAlign$^\dagger$} &                               & 27.6 & 14.8   & 27.9 & 32.4    & 27.9 & 16.2 & 29.3 & 30.8\\
\midrule
\midrule
Mask R-CNN 					 &	\multirow{2}{*}{R-101}  		& 20.9 &  3.1  &  19.4 & 29.9 & 21.3 & 3.5 & 21.1 & 28.9\\
Mask R-CNN$^\dagger$ 		 & 	                                & 20.9 &  3.1  &  19.4 & 29.9 & 21.3 & 3.5 & 21.1 & 28.9\\
%\midrule
RFS\cite{gupta2019lvis}  &  \multirow{2}{*}{R-101}	  & 23.5 & 11.3 & 22.3 & \textbf{29.9} & 24.1 & 11.6 & 23.9 & \textbf{29.3}\\
EQL\cite{gupta2019lvis}    & 	& - & - &  - & - & 24.4 & 14.5& 24.3 & 28.4 \\
\midrule
\textbf{DisAlign} &  \multirow{2}{*}{R-101}  \\
\textbf{DisAlign$^\dagger$} \\
\midrule
\midrule
Mask R-CNN 					&	\multirow{2}{*}{X-101} 		& 20.9 &  3.1  &  19.4 & 29.9 & 21.3 & 3.5 & 21.1 & 28.9\\
Mask R-CNN$^\dagger$ 	   &	 		& 20.9 &  3.1  &  19.4 & 29.9 & 21.3 & 3.5 & 21.1 & 28.9\\
\midrule
RFS\cite{gupta2019lvis}  &  \multirow{2}{*}{X-101}	  & 23.5 & 11.3 & 22.3 & \textbf{29.9} & 24.1 & 11.6 & 23.9 & \textbf{29.3}\\
EQL\cite{gupta2019lvis}    & 	& - & - &  - & - & 24.4 & 14.5& 24.3 & 28.4 \\
\midrule
+ \textbf{DisAlign} &  \multirow{2}{*}{X-101}  \\
+ \textbf{DisAlign$^\dagger$} \\
\bottomrule
\end{tabular}}

\end{table*}
